# Supplementary material for: Exact heat flux formula and its spectral decomposition in molecular dynamics for arbitrary many-body potentials
Source: arXiv:2509.26044 source file (2025-12-09)
Supplement: Supplementary file 1 [file Supplementary.pdf]

# Supplementary Material for: Accurate implementation of heat flux and its spectral decomposition in molecular dynamics for arbitrary many-body potentials

Markos Poulos,<sup>1</sup> Donatas Surblys,<sup>2</sup> and Konstantinos Termentzidis<sup>3</sup>

<sup>1</sup>*INSA Lyon, CNRS, CETHIL, UMR5008, 69621 Villeurbanne, France*

<sup>2</sup>*Institute of Fluid Science, Tohoku University,*

*2-1-1 Katahira, Aoba-ku, Sendai 980-8577, Japan*

<sup>3</sup>*CNRS, INSA Lyon, CETHIL, UMR5008, 69621 Villeurbanne, France*

## I. COMPUTATIONAL DETAILS

All systems were initially structurally and thermally relaxed at 300 K before the main simulations and are shown in Fig. S1. For all cases except a-SiO<sub>2</sub>, a universal timestep of  $dt=0.5$  fs was used both for the equilibration and the main simulations. For a-SiO<sub>2</sub> this timestep led to energy instability under the Tersoff potential that was used to model the interactions, so we used  $dt=0.25$  fs instead. With this value, the energy of the amorphous structure was found to be stable. The equilibration was performed first by static energy minimization under Conjugate Gradient (CG) optimization, followed by NPT volume relaxation and thermal equilibration for a total of 1 ns. This was done using a Nosé-Hoover thermostat with zero pressure and room temperature ( $T=300$  K) and relaxation time  $\tau=100*dt$ .

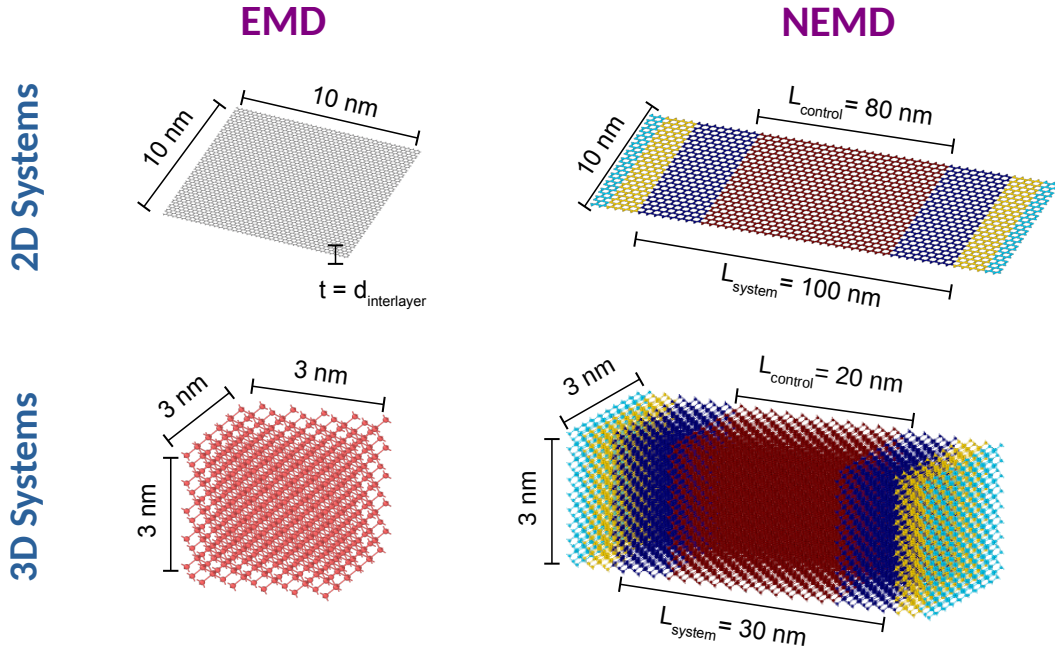

FIG. S1. Schematic of the configurations and geometries of all the systems used, whether 2D (top) or 3D (bottom). For the GK simulations (left) the systems were placed under Periodic Boundary Conditions. For the NEMD simulations (right) the systems were rectangular with fixed edges at the two ends (light blue), next to which the thermostat regions were placed (yellow), in to create a temperature gradient. The control volumes where the HF was calculated (red) were placed far from the thermostats. The control surfaces were simple cross-sections placed in the middle of the control volumes, perpendicular to the heat flow (not shown here).

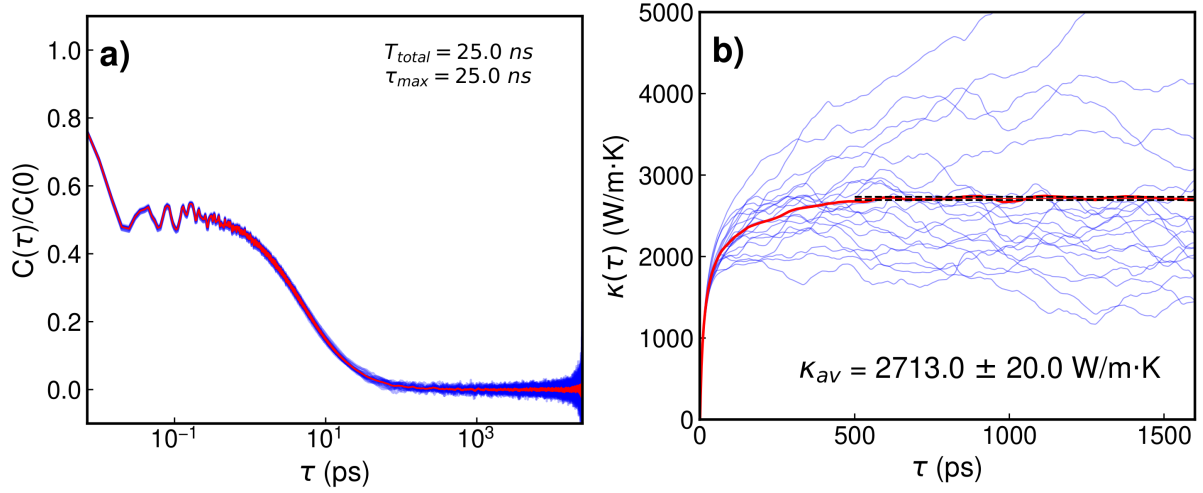

FIG. S2. Example of a GK calculation of  $\kappa$  for graphene at  $T=300$  K with the Tersoff-2010 potential. a) The normalized  $C(\tau)$  (average over  $C_{xx}$  and  $C_{yy}$ ), as a function of correlation time  $\tau$ , averaged over 20 independent simulations with different initial conditions, each running for  $T_{total}=25$  ns (*in blue*), as well as their ensemble average (*in red*). b) The running thermal conductivity  $\kappa(\tau)$  (average over  $\kappa_{xx}$  and  $\kappa_{yy}$ ) resulting from the integration of the individual curves in a) (*in blue*), as well as their ensemble average (*in red*). The final value  $\kappa_{av}$  is determined from the average of  $\kappa(\tau)$  for  $0.5 < \tau < 1.6$  ns.

For the Green-Kubo (GK) simulations, the systems were kept in equilibrium at room temperature  $T=300$  K under periodic boundary conditions. The 2D systems were square sheets of 10 nm in side, while the 3D systems were cubes of 5 nm on each side. We sampled the volume-averaged heat flux  $\mathbf{J}(t)$  both from the centroid formula eqs. (6)–(8) and from the group formula in eq. (9) and the thermal conductivity tensor  $\kappa_{ij}$  was then calculated from the standard GK equation:

$$\kappa_{ij} = \frac{1}{k_B T^2} \int_0^\infty \langle J_i(\tau) J_j(0) \rangle d\tau \quad (1)$$

where  $k_B$  is the Boltzmann constant, and  $\langle J(\tau)J(0) \rangle$  denotes a time autocorrelation function, henceforth denoted as  $C(\tau)$ . For the 3D systems we averaged over  $\kappa_{xx}$ ,  $\kappa_{yy}$  and  $\kappa_{zz}$ , while for the 2D systems we averaged over  $\kappa_{xx}$  and  $\kappa_{yy}$ . Sampling of  $\mathbf{J}(t)$  was done every  $\Delta t_{sample}=5$  fs, and for all cases besides 1LG the total simulation time was  $T_{total}=10$  ns, which was sufficient for  $C(\tau)$  to decay to zero. For 1LG, persistent oscillations of  $C(\tau)$  were observed, so for this case we used  $T_{total}=25$  ns. In order to reduce the noise in the integral of eq. (1), we averaged the results over 20 independent simulations with different initial conditions. All computational cells contained at least  $10^4$  atoms, which was sufficient to ensure that the results were converged with respect to the system size (see the relevant comparison in [1]). In Fig. S2 we show an example of these

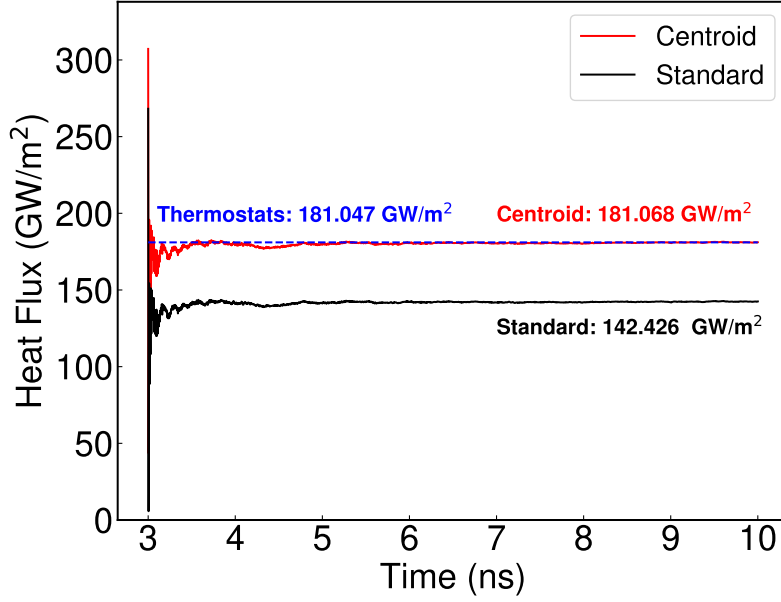

FIG. S3. Example of a NEMD calculation in 1LG, where the cumulative average of heat current  $Q$  is obtained by three distinct ways: i) From the thermostat energy exchange rate,  $Q_{thermo}$  (blue dashed horizontal line), ii) From the ‘centroid’ formula of HF in a control volume far from the heat baths with eqs. (6)–(8) (red), iii) From the ‘group’ formula of HF in a control volume far from the heat baths with eqs. (6)+(9) (black). The system is left to reach steady state for 3 ns and final values are obtained by averaging over 7 ns.

calculations for 1LG, both for  $C(\tau)$  and  $\kappa$ .

For the NEMD simulations, the systems were shaped as rectangles with a constant length  $L$  along the  $x$ -axis, and a constant temperature difference of  $\Delta T=60$  K was applied along  $L$  by connecting thermal reservoirs at the two ends. For the 2D systems  $L=100$  nm, while for the 3D systems  $L=50$  nm. The thermostat temperature was controlled using a Velocity Rescaling algorithm under fast dynamics (rescaling every 0.01 ps), while the average temperature was kept at  $T_0=300$  K. The edges of the systems were kept fixed to avoid drift, and periodic boundary conditions were applied perpendicular to the heat flux directions to simulate infinite width. For the 2D systems the boundary conditions along the cross-plane direction were kept non-periodic. The heat current  $Q$  was obtained both from the energy exchange rate of the thermostats, henceforth labeled  $Q_{thermo}$ , and from the heat flux inside a control volume from eq. (6), obtained as  $Q = J_x A_x$ , where  $J_x$  denotes the HF along the  $x$ -axis and  $A_x$  is the cross-section perpendicular to the heat flux direction (the  $x$ -axis).

Finally, for the spectral decomposition of  $Q$ , the fictitious interface was placed at the center

of the system, since both Tersoff and SW are short-range 3-body potentials, the summation over atoms in eq. (18) was restricted to  $\pm 3$  nm from the interface. Samples for  $\mathbf{F}_i^{1 \rightarrow 2}$  and  $\mathbf{v}_i$  were collected every  $\Delta t_{\text{sample}} = 5$  fs, for a total of  $T_{\text{total}} = 1$  ns, while data from 10 independent simulations with different initial conditions were obtained. The Fourier transform of the forces and velocities was performed using SciPy's FFT module [2]. In order to check for spectral leakage due to the finite length of the time series, we checked the results by using a Blackman window function, with no significant differences observed. The final spectra were smoothed using a Gaussian filter with FWHM of 0.1 THz for MoS<sub>2</sub> and 1 THz for 1LG.

- 
- [1] Z. Fan, T. Siro, and A. Harju, Force and heat current formulas for many-body potentials in molecular dynamics simulations with applications to thermal conductivity calculations, *Physical Review B* **91**, 094301 (2015).
  - [2] P. Virtanen, R. Gommers, T. E. Oliphant, M. Haberland, T. Reddy, D. Cournapeau, E. Burovski, P. Peterson, W. Weckesser, J. Bright, S. J. van der Walt, M. Brett, J. Wilson, K. J. Millman, N. Mayorov, A. R. J. Nelson, E. Jones, R. Kern, E. Larson, C. J. Carey, Í. Polat, Y. Feng, E. W. Moore, J. VanderPlas, D. Laxalde, J. Perktold, R. Cimrman, I. Henriksen, E. A. Quintero, C. R. Harris, A. M. Archibald, A. H. Ribeiro, F. Pedregosa, P. van Mulbregt, and SciPy 1.0 Contributors, SciPy 1.0: Fundamental Algorithms for Scientific Computing in Python, *Nature Methods* **17**, 261 (2020).
